# Supplementary material for: OneFlow: Concurrent Mixed-Modal and Interleaved Generation with Edit Flows
Source: arXiv:2510.03506 source file (2025-12-10)
Supplement: Supplementary file 1 [file color_example_appendix.tex]

\begin{table}
\begin{tabular}{m{0.74\linewidth} m{0.18\linewidth}}
\toprule
\multicolumn{2}{l}{
Generated tokens: $t=0$ \colorbox[HTML]{5c469d}{\rule{0.0em}{1em}}\colorbox[HTML]{686cad}{\rule{0.0em}{1em}}\colorbox[HTML]{7493bd}{\rule{0.0em}{1em}}\colorbox[HTML]{80bacd}{\rule{0.0em}{1em}}\colorbox[HTML]{8ce1dd}{\rule{0.0em}{1em}}\colorbox[HTML]{99fde7}{\rule{0.0em}{1em}}\colorbox[HTML]{a9f6df}{\rule{0.0em}{1em}}\colorbox[HTML]{b8efd6}{\rule{0.0em}{1em}}\colorbox[HTML]{c7e9cd}{\rule{0.0em}{1em}}\colorbox[HTML]{d7e2c5}{\rule{0.0em}{1em}}\colorbox[HTML]{e2c7b6}{\rule{0.0em}{1em}}\colorbox[HTML]{e998a1}{\rule{0.0em}{1em}}\colorbox[HTML]{ef698c}{\rule{0.0em}{1em}}\colorbox[HTML]{f63a78}{\rule{0.0em}{1em}}\colorbox[HTML]{fd0b63}{\rule{0.0em}{1em}}\colorbox[HTML]{e80756}{\rule{0.0em}{1em}}\colorbox[HTML]{ca104b}{\rule{0.0em}{1em}}\colorbox[HTML]{ac1a41}{\rule{0.0em}{1em}}\colorbox[HTML]{8e2337}{\rule{0.0em}{1em}}\colorbox[HTML]{702d2d}{\rule{0.0em}{1em}} $t=1$
} \\
\midrule
{\color[HTML]{000000}What} {\color[HTML]{000000}is} {\color[HTML]{000000}the} {\color[HTML]{000000}Bac} {\color[HTML]{000000}Son} {\color[HTML]{000000}Valley}{\color[HTML]{000000}?} {\color[HTML]{000000}can} {\color[HTML]{000000}you} {\color[HTML]{000000}show} {\color[HTML]{000000}me} {\color[HTML]{000000}an} {\color[HTML]{000000}image}{\color[HTML]{000000}?} {\color[HTML]{97fee9}Sure}{\color[HTML]{5c469d},} {\color[HTML]{5c469d}here}{\color[HTML]{5c469d}'s} {\color[HTML]{8f2337}an} {\color[HTML]{6460a8}image} {\color[HTML]{f63c78}of} {\color[HTML]{a4f8e1}the} {\color[HTML]{d0e5c9}Bac} {\color[HTML]{97fee9}Son} {\color[HTML]{6668ab}Valley}{\color[HTML]{5d4b9f}:}{\color[HTML]{6054a3}\textless{}\textbar{}image\textbar{}\textgreater{}}{\color[HTML]{b7f0d7}B}{\color[HTML]{84c5d2}ac} {\color[HTML]{e1d0ba}Son} {\color[HTML]{ee0558}Valley}{\color[HTML]{ee0558},} {\color[HTML]{7595be}also} {\color[HTML]{702d2d}known} {\color[HTML]{b7f0d7}as} {\color[HTML]{84c5d2}the} {\color[HTML]{6460a8}Bach} {\color[HTML]{bdedd3}Ma} {\color[HTML]{85c9d3}National} {\color[HTML]{fe0660}Park}{\color[HTML]{5d4b9f},} {\color[HTML]{a1fae3}is} {\color[HTML]{c5eacf}a} {\color[HTML]{d10e4e}scenic} {\color[HTML]{9d1e3c}and} {\color[HTML]{6460a8}culturally} {\color[HTML]{e0d1ba}rich} {\color[HTML]{625aa5}region} {\color[HTML]{8ce1dd}located} {\color[HTML]{5e4c9f}in} {\color[HTML]{fd0c63}central} {\color[HTML]{79a2c3}Vietnam}{\color[HTML]{f9286f}.} {\color[HTML]{f15c87}It} {\color[HTML]{6155a3}is} {\color[HTML]{e5b3ad}situated} {\color[HTML]{c5eacf}in} {\color[HTML]{6054a3}the} {\color[HTML]{eb899b}provinces} {\color[HTML]{e0d1ba}of} {\color[HTML]{d30d4e}Th}{\color[HTML]{6155a3}ua} {\color[HTML]{5d4b9f}Th}{\color[HTML]{e9939f}ien}{\color[HTML]{6668ab}-H}{\color[HTML]{9afde7}ue} {\color[HTML]{892435}and} {\color[HTML]{9afde7}Quang} {\color[HTML]{cc0f4c}Nam}{\color[HTML]{da0b51},} {\color[HTML]{c2ebd0}about}{\color[HTML]{5e4c9f}50} {\color[HTML]{a7f7e0}kilometres} {\color[HTML]{752b2e}southwest} {\color[HTML]{6460a8}of} {\color[HTML]{beedd3}Hue} {\color[HTML]{92f5e5}City}{\color[HTML]{c0ecd1}.} {\color[HTML]{6a73af}The} {\color[HTML]{6668ab}valley} {\color[HTML]{88d4d8}stretches} {\color[HTML]{8ee8e0}for} {\color[HTML]{6054a3}approximately}{\color[HTML]{7085b7}50} {\color[HTML]{d2e4c7}kilometres} {\color[HTML]{f63c78}in} {\color[HTML]{78a0c2}southwest} {\color[HTML]{ee0558}and} {\color[HTML]{92f5e5}stretches} {\color[HTML]{c0ecd1}for} {\color[HTML]{6155a3}about}{\color[HTML]{6a73af}20} {\color[HTML]{5e4c9f}kilometres} {\color[HTML]{f63c78}southwest} {\color[HTML]{78a0c2}of} {\color[HTML]{beedd3}Hue} {\color[HTML]{f82e72}City}{\color[HTML]{c0ecd1}.} {\color[HTML]{6a73af}The} {\color[HTML]{6668ab}valley} {\color[HTML]{88d4d8}is} {\color[HTML]{8ee8e0}surrounded} {\color[HTML]{6054a3}by} {\color[HTML]{7085b7}mountains} {\color[HTML]{d2e4c7}on} {\color[HTML]{e0d1ba}all} {\color[HTML]{7a2930}sides}{\color[HTML]{f9246e},} {\color[HTML]{fc0d64}creating} {\color[HTML]{f82f72}a} {\color[HTML]{5d4b9f}unique} {\color[HTML]{f73776}micro}{\color[HTML]{6460a8}climate} {\color[HTML]{e4b8b0}that} {\color[HTML]{625aa5}stretches} {\color[HTML]{f06289}on} {\color[HTML]{718bba}all} {\color[HTML]{e89aa2}sides}{\color[HTML]{85c9d3},} {\color[HTML]{f63c78}creating} {\color[HTML]{f82f72}a} {\color[HTML]{5d4b9f}unique} {\color[HTML]{f73776}micro}{\color[HTML]{6460a8}climate} {\color[HTML]{e4b8b0}that} {\color[HTML]{625aa5}supports} {\color[HTML]{f06289}a} {\color[HTML]{718bba}diverse} {\color[HTML]{e89aa2}range} {\color[HTML]{85c9d3}of} {\color[HTML]{932139}flora} {\color[HTML]{625aa5}and} {\color[HTML]{9b1f3b}fauna}{\color[HTML]{86ced5}.}{\color[HTML]{6668ab}B}{\color[HTML]{c9e8cd}ac} {\color[HTML]{5e4c9f}Son} {\color[HTML]{e0d2bb}Valley} {\color[HTML]{6054a3}is} {\color[HTML]{7595be}home} {\color[HTML]{702d2d}to} {\color[HTML]{b7f0d7}many} {\color[HTML]{84c5d2}ethnic} {\color[HTML]{e0d1ba}minority} {\color[HTML]{5c469d}groups}{\color[HTML]{5c469d},} {\color[HTML]{5c469d}including} {\color[HTML]{7699bf}the} {\color[HTML]{5c469d}Tay}{\color[HTML]{5c469d},} {\color[HTML]{6460a8}N}{\color[HTML]{5c469d}ung}{\color[HTML]{5d4b9f},} {\color[HTML]{769bc0}and} {\color[HTML]{6460a8}Hoa} {\color[HTML]{5c469d}communities}{\color[HTML]{bdedd3},} {\color[HTML]{6460a8}who} {\color[HTML]{5e4c9f}have} {\color[HTML]{6e81b5}lived} {\color[HTML]{91f0e3}there} {\color[HTML]{6460a8}for} {\color[HTML]{676bac}centuries} {\color[HTML]{5c469d}and} {\color[HTML]{5c469d}maintain} {\color[HTML]{baeed5}their} {\color[HTML]{78a0c2}traditional} {\color[HTML]{7fb7cc}ways} {\color[HTML]{5e4c9f}of} {\color[HTML]{5c469d}life}{\color[HTML]{5c469d}.} {\color[HTML]{5c469d}Visitors} {\color[HTML]{5c469d}can} {\color[HTML]{6668ab}experience} {\color[HTML]{5c469d}the} {\color[HTML]{6054a3}local} {\color[HTML]{5c469d}culture} {\color[HTML]{5c469d}by} {\color[HTML]{6a73b0}visiting} {\color[HTML]{5d4b9f}villages}{\color[HTML]{779ec1},} {\color[HTML]{5c489e}participating} {\color[HTML]{f9246e}in} {\color[HTML]{5c469d}festivals}{\color[HTML]{5c469d},} {\color[HTML]{6460a8}and} {\color[HTML]{82c0d0}learning} {\color[HTML]{6155a3}about} {\color[HTML]{5c469d}the} {\color[HTML]{6460a8}customs} {\color[HTML]{5e4c9f}and} {\color[HTML]{5c469d}traditions} {\color[HTML]{beedd3}of} {\color[HTML]{5d4b9f}these} {\color[HTML]{8de2de}communities}{\color[HTML]{5e4c9f}.}{\color[HTML]{acf5dd}The} {\color[HTML]{6668ab}valley}{\color[HTML]{5c469d}'s} {\color[HTML]{91f0e3}main} {\color[HTML]{6054a3}attractions}{\color[HTML]{5c469d},} {\color[HTML]{d2e4c7}the} {\color[HTML]{a4f8e1}Bac} {\color[HTML]{5c469d}Son} {\color[HTML]{5c469d}Valley}{\color[HTML]{6460a8},} {\color[HTML]{5d4b9f}which} {\color[HTML]{6054a3}is} {\color[HTML]{b7f0d7}known} {\color[HTML]{84c5d2}for} {\color[HTML]{6460a8}its} {\color[HTML]{5c469d}natural} {\color[HTML]{e0d1ba}beauty} {\color[HTML]{85c9d3}and} {\color[HTML]{78a0c2}rural} {\color[HTML]{91f1e4}traditions}{\color[HTML]{5c469d}.} {\color[HTML]{5c469d}The} {\color[HTML]{5e4c9f}valley} {\color[HTML]{5c469d}is} {\color[HTML]{acf5dd}home} {\color[HTML]{6054a3}to} {\color[HTML]{7085b7}many} {\color[HTML]{d2e4c7}ethnic} {\color[HTML]{e0d1ba}minority} {\color[HTML]{5c469d}groups}{\color[HTML]{5c469d},} {\color[HTML]{5c469d}including} {\color[HTML]{7699bf}the} {\color[HTML]{5c469d}Tay}{\color[HTML]{5c469d},} {\color[HTML]{6460a8}N}{\color[HTML]{5c469d}ung}{\color[HTML]{5d4b9f},} {\color[HTML]{769bc0}and} {\color[HTML]{6460a8}Hoa} {\color[HTML]{5c469d}communities}{\color[HTML]{bdedd3},} {\color[HTML]{6460a8}who} {\color[HTML]{5e4c9f}have} {\color[HTML]{6e81b5}lived} {\color[HTML]{91f0e3}there} {\color[HTML]{6460a8}for} {\color[HTML]{676bac}centuries} {\color[HTML]{5c469d}and} {\color[HTML]{5c469d}their} {\color[HTML]{baeed5}traditional} {\color[HTML]{78a0c2}ways} {\color[HTML]{7fb7cc}of} {\color[HTML]{5e4c9f}life}{\color[HTML]{5c469d}.} {\color[HTML]{5c469d}The} {\color[HTML]{5c469d}valley} {\color[HTML]{6668ab}is} {\color[HTML]{5c469d}also} {\color[HTML]{6054a3}known} {\color[HTML]{7085b7}for} {\color[HTML]{d2e4c7}its} {\color[HTML]{e0d1ba}natural} {\color[HTML]{bdedd3}beauty}{\color[HTML]{85c9d3},} {\color[HTML]{78a0c2}with} {\color[HTML]{91f1e4}lush} {\color[HTML]{5c469d}green} {\color[HTML]{5c469d}fields}{\color[HTML]{6460a8},} {\color[HTML]{c3ead0}beautiful} {\color[HTML]{5c469d}limestone} {\color[HTML]{a6f7e0}cliffs}{\color[HTML]{5c469d},} {\color[HTML]{6460a8}terr}{\color[HTML]{86cdd5}aced} {\color[HTML]{5c469d}fields}{\color[HTML]{5c469d},} {\color[HTML]{6460a8}terr}{\color[HTML]{a4f8e1}aced} {\color[HTML]{6e82b6}fields}{\color[HTML]{5c469d},} {\color[HTML]{6460a8}and} {\color[HTML]{a4f8e1}towering} {\color[HTML]{6e82b6}limestone} {\color[HTML]{5c469d}cliffs} {\color[HTML]{6460a8}rising} {\color[HTML]{5e4c9f}from} {\color[HTML]{5c469d}the} {\color[HTML]{5c469d}river}{\color[HTML]{5c469d}banks}{\color[HTML]{5c469d}.} {\color[HTML]{5c469d}The} {\color[HTML]{5d4b9f}main} {\color[HTML]{779cc0}river} {\color[HTML]{bbeed5}flowing} {\color[HTML]{6054a3}through} {\color[HTML]{7085b7}the} {\color[HTML]{5c469d}Bac} {\color[HTML]{779cc0}Son} {\color[HTML]{5c469d}river} {\color[HTML]{5c469d}is} {\color[HTML]{5d4b9f}the} {\color[HTML]{6054a3}Bac} {\color[HTML]{b7f0d7}Son} {\color[HTML]{779cc0}River}{\color[HTML]{e0d1ba},} {\color[HTML]{5d4b9f}which} {\color[HTML]{6054a3}offers} {\color[HTML]{b7f0d7}stunning} {\color[HTML]{5c469d}views} {\color[HTML]{6460a8}and} {\color[HTML]{5c469d}beautiful} {\color[HTML]{5c469d}views}{\color[HTML]{5c469d},} {\color[HTML]{5c469d}as} {\color[HTML]{5e4c9f}well} {\color[HTML]{86cdd5}as} {\color[HTML]{5c469d}opportunities} {\color[HTML]{6460a8}for} {\color[HTML]{fe0660}kay}{\color[HTML]{5c469d}aking} {\color[HTML]{fe0660}and} {\color[HTML]{5c469d}fishing}{\color[HTML]{78a0c2}.} {\color[HTML]{6052a2}The} {\color[HTML]{6b78b2}Other} {\color[HTML]{5e4c9f}attractions} {\color[HTML]{5c469d}include} {\color[HTML]{6054a3}the} {\color[HTML]{7085b7}Bac} {\color[HTML]{5c469d}Son} {\color[HTML]{5c469d}Valley}{\color[HTML]{635ea7}'s} {\color[HTML]{5d4b9f}natural} {\color[HTML]{6054a3}beauty}{\color[HTML]{b7f0d7},} {\color[HTML]{84c5d2}which} {\color[HTML]{a4f8e1}include} {\color[HTML]{5c469d}lush} {\color[HTML]{5c469d}green} {\color[HTML]{6460a8}rice} {\color[HTML]{5c469d}padd}{\color[HTML]{635ea7}ies}{\color[HTML]{5c469d},} {\color[HTML]{a6f7e0}terr}{\color[HTML]{5c469d}aced} {\color[HTML]{5c469d}fields}{\color[HTML]{5c469d},} {\color[HTML]{6460a8}and} {\color[HTML]{a4f8e1}water}{\color[HTML]{6e82b6}falls}{\color[HTML]{5c469d}.} {\color[HTML]{6460a8}Other} {\color[HTML]{5e4c9f}attractions} {\color[HTML]{5c469d}include} {\color[HTML]{6e80b5}caves}{\color[HTML]{6054a3},} {\color[HTML]{5c469d}water}{\color[HTML]{5c469d}falls}{\color[HTML]{635ea7},} {\color[HTML]{5c469d}and} {\color[HTML]{6460a8}ancient} {\color[HTML]{5c469d}temples}{\color[HTML]{6e80b5},} {\color[HTML]{6460a8}such} {\color[HTML]{5e4c9f}as} {\color[HTML]{7aa8c5}the} {\color[HTML]{99fde7}Linh} {\color[HTML]{6460a8}Ung} {\color[HTML]{5c469d}Pag}{\color[HTML]{fe0660}oda} {\color[HTML]{5d4b9f}and} {\color[HTML]{5c469d}the} {\color[HTML]{7493bd}Ph}{\color[HTML]{82c0d0}ap} {\color[HTML]{5d499e}Lam} {\color[HTML]{5e4c9f}Pag}{\color[HTML]{5d4b9f}oda}{\color[HTML]{8de4de}.}{\color[HTML]{5c469d}Overall}{\color[HTML]{5c469d},} {\color[HTML]{82c0d0}Bac} {\color[HTML]{5d499e}Son} {\color[HTML]{6054a3}Valley} {\color[HTML]{5c469d}is} {\color[HTML]{6460a8}a} {\color[HTML]{6054a3}must}{\color[HTML]{b7f0d7}-}{\color[HTML]{84c5d2}visit} {\color[HTML]{e0d1ba}destination} {\color[HTML]{625aa5}for} {\color[HTML]{5c469d}anyone} {\color[HTML]{5c469d}interested} {\color[HTML]{5c469d}in} {\color[HTML]{5c469d}exploring} {\color[HTML]{78a0c2}rural} {\color[HTML]{5f50a1}Vietnamese} {\color[HTML]{5c469d}culture} {\color[HTML]{6155a3}and} {\color[HTML]{5c469d}experiencing} {\color[HTML]{5c469d}the} {\color[HTML]{5c469d}country}{\color[HTML]{5c489e}'s} {\color[HTML]{5e4c9f}natural} {\color[HTML]{5c469d}beauty}{\color[HTML]{5d4b9f}.}
&
\includegraphics[width=1.0\linewidth]{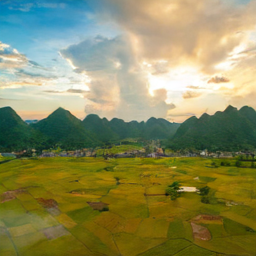}
\\
\midrule
{\color[HTML]{000000}What} {\color[HTML]{000000}are} {\color[HTML]{000000}the} {\color[HTML]{000000}largest} {\color[HTML]{000000}const}{\color[HTML]{000000}ell}{\color[HTML]{000000}ations} {\color[HTML]{000000}in} {\color[HTML]{000000}the} {\color[HTML]{000000}night} {\color[HTML]{000000}sky}{\color[HTML]{000000}?} {\color[HTML]{000000}Include} {\color[HTML]{000000}pictures} {\color[HTML]{000000}and} {\color[HTML]{000000}tell} {\color[HTML]{000000}me} {\color[HTML]{000000}how} {\color[HTML]{000000}much} {\color[HTML]{000000}space} {\color[HTML]{000000}they} {\color[HTML]{000000}take} {\color[HTML]{000000}up} {\color[HTML]{000000}in} {\color[HTML]{000000}the} {\color[HTML]{000000}sky}{\color[HTML]{000000},} {\color[HTML]{000000}please}{\color[HTML]{000000}.} {\color[HTML]{5c469d}Sure}{\color[HTML]{769ac0}!} {\color[HTML]{5c469d}Here} {\color[HTML]{5c469d}are} {\color[HTML]{f15a86}the} {\color[HTML]{7390bc}largest} {\color[HTML]{fe005e}const}{\color[HTML]{d4e3c6}ell}{\color[HTML]{9bfce6}ations} {\color[HTML]{6d7db4}and} {\color[HTML]{99fde8}some} {\color[HTML]{d6e2c5}info} {\color[HTML]{cbe7cc}on} {\color[HTML]{9bfce7}them}{\color[HTML]{e3beb2},} {\color[HTML]{702d2d}along} {\color[HTML]{ec0557}with} {\color[HTML]{c3ebd0}pictures}{\color[HTML]{7391bc}.}{\color[HTML]{ce0f4d}The} {\color[HTML]{a5f8e1}three} {\color[HTML]{90ede2}largest} {\color[HTML]{769ac0}const}{\color[HTML]{f73776}ell}{\color[HTML]{5c469d}ations} {\color[HTML]{6d7db4}you} {\color[HTML]{99fde8}might} {\color[HTML]{d6e2c5}find} {\color[HTML]{cbe7cc}in} {\color[HTML]{dfd8be}the} {\color[HTML]{9bfce6}night} {\color[HTML]{5c469d}sky}{\color[HTML]{5c479d},} {\color[HTML]{9bfce6}along} {\color[HTML]{9ffbe4}with} {\color[HTML]{7cadc7}some} {\color[HTML]{7391bc}info} {\color[HTML]{ce0f4d}on} {\color[HTML]{a5f8e1}them}{\color[HTML]{e3beb2},} {\color[HTML]{702d2d}are} {\color[HTML]{ec0557}the} {\color[HTML]{c3ebd0}Hydra}{\color[HTML]{7391bc},} {\color[HTML]{d4e3c6}Vir}{\color[HTML]{9bfce6}go}{\color[HTML]{6c79b2},} {\color[HTML]{7391bc}and} {\color[HTML]{5c469d}U}{\color[HTML]{5c469d}rsa} {\color[HTML]{7391bc}Major}{\color[HTML]{9bfce7}.}{\color[HTML]{c2ebd0}Here}{\color[HTML]{6970ae}'s} {\color[HTML]{7fb7cc}some} {\color[HTML]{769ac0}pictures} {\color[HTML]{cbe7cb}of} {\color[HTML]{5d499e}the} {\color[HTML]{e3beb2}largest} {\color[HTML]{90ede2}const}{\color[HTML]{5e4ea0}ell}{\color[HTML]{9bfce6}ations}{\color[HTML]{6d7db4},} {\color[HTML]{99fde8}along} {\color[HTML]{d6e2c5}with} {\color[HTML]{cbe7cc}pictures} {\color[HTML]{7391bc}about} {\color[HTML]{ce0f4d}them}{\color[HTML]{a5f8e1}:}{\color[HTML]{90ede2}1}{\color[HTML]{7aa7c5}.} {\color[HTML]{c3ebd0}Hydra}{\color[HTML]{728cba}:} {\color[HTML]{eb8a9b}The} {\color[HTML]{769ac0}Hydra} {\color[HTML]{6c79b2}constellation} {\color[HTML]{728cba}is} {\color[HTML]{99fde7}the} {\color[HTML]{6c79b2}largest} {\color[HTML]{fb1667}in} {\color[HTML]{5c469d}the} {\color[HTML]{9bfce6}night} {\color[HTML]{6d7db4}sky}{\color[HTML]{5c479d},} {\color[HTML]{9bfce6}taking} {\color[HTML]{9ffbe4}up} {\color[HTML]{7cadc7}about}{\color[HTML]{7391bc}3}{\color[HTML]{f9236d}.}{\color[HTML]{b8efd6}16}{\color[HTML]{7aa7c5}\%} {\color[HTML]{6a72af}of} {\color[HTML]{769ac0}the} {\color[HTML]{f63977}visible} {\color[HTML]{7dafc8}sky}{\color[HTML]{5e4ea0}.}{\color[HTML]{9bfce6}Here}{\color[HTML]{83c5d1}'s} {\color[HTML]{7cadc7}a} {\color[HTML]{769ac0}picture} {\color[HTML]{cbe7cb}of} {\color[HTML]{5d499e}the} {\color[HTML]{5c469d}Hydra} {\color[HTML]{5c469d}constellation}{\color[HTML]{5e4ea0}:}{\color[HTML]{9bfce6}\textless{}\textbar{}image\textbar{}\textgreater{}}{\color[HTML]{6c79b2}3}{\color[HTML]{fb1667}.} {\color[HTML]{728cba}U}{\color[HTML]{5c469d}rsa} {\color[HTML]{5c469d}Major}{\color[HTML]{6a72af}:} {\color[HTML]{769ac0}The} {\color[HTML]{c2ebd0}U}{\color[HTML]{6970ae}rsa} {\color[HTML]{7fb7cc}Major} {\color[HTML]{728cba}is} {\color[HTML]{99fde7}the} {\color[HTML]{c2ebd0}third} {\color[HTML]{6970ae}largest} {\color[HTML]{7fb7cc}constellation}{\color[HTML]{5c469d},} {\color[HTML]{9bfce6}covering} {\color[HTML]{5c469d}about}{\color[HTML]{6d7db4}3}{\color[HTML]{fb1667}.}{\color[HTML]{7391bc}1}{\color[HTML]{5c469d}\%} {\color[HTML]{7aa7c5}of} {\color[HTML]{6a72af}the} {\color[HTML]{769ac0}night} {\color[HTML]{eb8a9b}sky}{\color[HTML]{7dafc8}.}{\color[HTML]{5e4ea0}Here}{\color[HTML]{9bfce6}'s} {\color[HTML]{9ffbe4}a} {\color[HTML]{7cadc7}picture} {\color[HTML]{769ac0}of} {\color[HTML]{cbe7cb}the} {\color[HTML]{5d499e}U}{\color[HTML]{5c469d}rsa} {\color[HTML]{5c469d}Major} {\color[HTML]{5e4ea0}constellation}{\color[HTML]{9bfce6}:}{\color[HTML]{c2ebd0}\textless{}\textbar{}image\textbar{}\textgreater{}}{\color[HTML]{6970ae}Here}{\color[HTML]{7fb7cc}'s} {\color[HTML]{fb1667}a} {\color[HTML]{728cba}picture} {\color[HTML]{5c469d}of} {\color[HTML]{5c469d}the} {\color[HTML]{cbe7cb}U}{\color[HTML]{5d499e}rsa} {\color[HTML]{5c469d}Major} {\color[HTML]{5c469d}constellation}{\color[HTML]{5e4ea0}:}{\color[HTML]{9bfce6}\textless{}\textbar{}image\textbar{}\textgreater{}}
&
\includegraphics[width=1.0\linewidth]{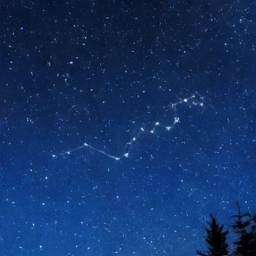}
\includegraphics[width=1.0\linewidth]{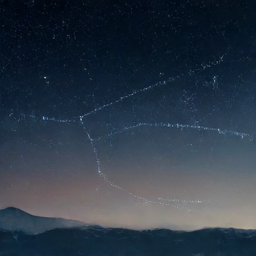}
\includegraphics[width=1.0\linewidth]{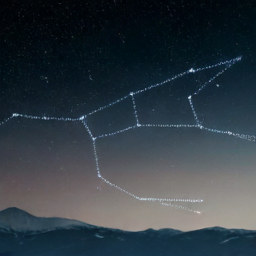}
\\
\midrule
{\color[HTML]{000000}I} {\color[HTML]{000000}am} {\color[HTML]{000000}taking} {\color[HTML]{000000}a} {\color[HTML]{000000}pottery} {\color[HTML]{000000}class} {\color[HTML]{000000}and} {\color[HTML]{000000}just} {\color[HTML]{000000}finished} {\color[HTML]{000000}my} {\color[HTML]{000000}first} {\color[HTML]{000000}piece} {\color[HTML]{000000}(}{\color[HTML]{000000}a} {\color[HTML]{000000}decorative} {\color[HTML]{000000}plate}{\color[HTML]{000000}).} {\color[HTML]{000000}I} {\color[HTML]{000000}need} {\color[HTML]{000000}some} {\color[HTML]{000000}inspiration} {\color[HTML]{000000}for} {\color[HTML]{000000}painting} {\color[HTML]{000000}it}{\color[HTML]{000000}.} {\color[HTML]{000000}Can} {\color[HTML]{000000}you} {\color[HTML]{000000}give} {\color[HTML]{000000}me} {\color[HTML]{000000}a} {\color[HTML]{000000}picture} {\color[HTML]{000000}that} {\color[HTML]{000000}I} {\color[HTML]{000000}could} {\color[HTML]{000000}use} {\color[HTML]{000000}as} {\color[HTML]{000000}inspiration}{\color[HTML]{000000}?} {\color[HTML]{000000}I} {\color[HTML]{000000}love} {\color[HTML]{000000}the} {\color[HTML]{000000}Moroccan} {\color[HTML]{000000}style}{\color[HTML]{000000}.} {\color[HTML]{ef6a8d}Congratulations} {\color[HTML]{f63977}on} {\color[HTML]{5c469d}creating} {\color[HTML]{5c469d}your} {\color[HTML]{f73776}first} {\color[HTML]{a41c3e}piece}{\color[HTML]{a21d3e}!} {\color[HTML]{d4e3c6}The} {\color[HTML]{e3c0b3}image} {\color[HTML]{6e81b5}below} {\color[HTML]{728ebb}might} {\color[HTML]{f10459}inspire} {\color[HTML]{c21349}you} {\color[HTML]{e4b7af}creating} {\color[HTML]{9cfce6}your} {\color[HTML]{f0678b}first} {\color[HTML]{91f1e4}piece}{\color[HTML]{a21d3e}.} {\color[HTML]{d4e3c6}The} {\color[HTML]{e3c0b3}image} {\color[HTML]{6e81b5}below} {\color[HTML]{f63977}might} {\color[HTML]{f10459}inspire} {\color[HTML]{c21349}you}{\color[HTML]{e4b7af}.} {\color[HTML]{f63977}\textless{}\textbar{}image\textbar{}\textgreater{}}{\color[HTML]{ec7e96}The} {\color[HTML]{c4eacf}Moroccan} {\color[HTML]{c4eacf}style} {\color[HTML]{932139}is} {\color[HTML]{932139}indeed} {\color[HTML]{f5407a}breathtaking}{\color[HTML]{d5e3c6}.} {\color[HTML]{ef6a8d}The} {\color[HTML]{8feae1}intricate} {\color[HTML]{702d2d}designs} {\color[HTML]{93f7e7}are} {\color[HTML]{f63977}a} {\color[HTML]{f10459}true} {\color[HTML]{ef6e8e}work} {\color[HTML]{782a30}of} {\color[HTML]{95fce8}art}{\color[HTML]{d4e3c6},} {\color[HTML]{ec0557}with} {\color[HTML]{eb879a}a} {\color[HTML]{c8e9cd}rich} {\color[HTML]{c9e8cd}history} {\color[HTML]{9bfce6}that} {\color[HTML]{6d7cb3}spans} {\color[HTML]{d4e3c6}centuries}{\color[HTML]{f63977}.}
& 
\includegraphics[width=1.0\linewidth]{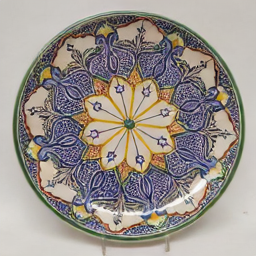}
\\

\bottomrule
\end{tabular}
\caption{OneFlow is able to generate text and images jointly. This example shows the timestep at which each token (including the image) is inserted at. Note that the image is first inserted as pure noise and progressively denoised along with the text. The image denoising is shown in Appendix \ref{sec:further_interleaved}.}
\label{tab:color_coded_example}
\end{table}
